# Supplementary material for: Constrained Non-Affine Alignment of Embeddings
Source: arXiv:1910.05862 source file (2021-11-19)
Supplement: Supplementary file 1 [file appendix.tex]

\clearpage

\appendix

{\LARGE Supplementary Material}

%\section{Details in Multi-Label Feature Removal}
\section{More Experiments on Imbalanced Multi-Label Synthetic Dataset}
\label{sec:multi-label}
As mentioned, the feature evaluation method can be directly extended to multiple categories of features. In this section, we demonstrate that the feature attenuation method can be extended as well.  

%\subsection{Multi-label Embedding Mapping}
Recall that the key to removing a binary categorical feature from a set of embeddings is separating the embeddings into two classes according to their feature values, and take these two classes as source domain and target domain respectively. We will extend this idea to multi-label scenarios where a given feature can take $M$ distinct values, and therefore we will have $M$ classes of embeddings. There are two possible solutions: a) we arbitrarily choose one class as the target domain and the rest $M-1$ classes as the source domains. In this case, we can learn $M-1$ mapping functions to map multiple source domains to the target domain independently; b) we choose one class as the target domain, and then map all the $M-1$ source domains together using one shared mapping function. In this work, we apply the first solution to the multi-label dataset and leave the second one as our further work.

\begin{table}[b]
\caption{Results on imbalanced synthetic multi-label dataset. We report the AUC for lightness (F1) and color (F2). }
\centering
%\resizebox{0.95\textwidth}{!}{ % If your table exceeds the column or page width, use this command to reduce it slightly
\begin{tabular}{l||c|c}
\hline
 & F1\_AUC  &  F2\_AUC\\ 
\hline
Raw data         &  0.98 &  0.81 \\
Green\_Target   & 0.98  &  0.77 \\
Red\_Target     &  0.98 &  0.64 \\
\hline
\end{tabular}
\label{table_binary_imbalance_multi}
\vspace{-5mm}
\end{table}

% \begin{figure}[htb]
%     \centering % <-- added
%     \subfigure[original]{\includegraphics[width=0.15\textwidth]{figs/synm1_org.png}} 
%     \subfigure[Orange as target domain]{\includegraphics[width=0.15\textwidth]{figs/synm1_g1.png}}
%     \subfigure[Blue as target domain]{\includegraphics[width=0.15\textwidth]{figs/synm1_g2.png}}
%     \caption{Imbalanced Synthetic data with binary label}
%     \label{fig:syn_multi_imbalance}
% \end{figure}
\begin{figure}[b]
    \centering
    \begin{subfigure}[b]{0.22\textwidth}
        \centering
        \includegraphics[width=\textwidth]{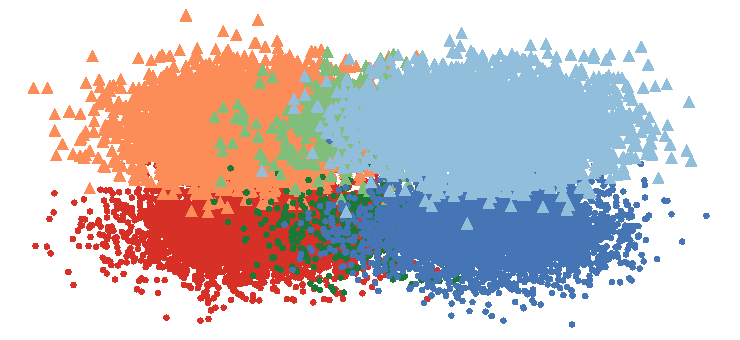}
        \caption{Raw data}
    \end{subfigure}
    
    \begin{subfigure}[b]{0.22\textwidth}
        \centering
        \includegraphics[width=\textwidth]{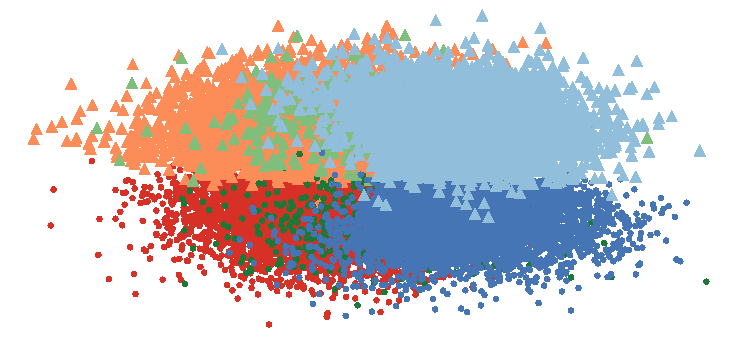}
        \caption{Green as target domain}
    \end{subfigure}
    \begin{subfigure}[b]{0.22\textwidth}
        \centering
        \includegraphics[width=\textwidth]{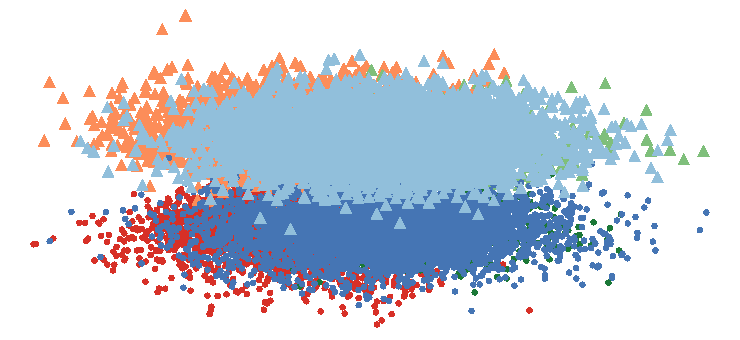}
        \caption{Red as target domain}
    \end{subfigure}
    \caption{Imbalanced multi-label synthetic dataset.}
    \label{fig:syn_multi_imbalance}
\end{figure}

%\subsubsection{Experiments on Imbalanced Multi-Label Synthetic Dataset}
We continue our experiments with the synthetic datasets. The visualization of the multi-label dataset is the same as the binary dataset: the x-axis varies with Feature 1 (F1) which is the color feature, and the y-axis varies with Feature 2 (F2) which is the lightness feature. There are still two classes for the lightness feature (light and dark), but now we have three classes for the color feature (green, red and blue).
To reduce the color feature, we can fix one color as the target domain and the other two colors as the source domains. 
For the balanced dataset, the choice of color as the target domain does not affect the results.
However, for the imbalanced case where there are $1,000$ green points, $10,000$ red points and $10,000$ blue points (illustrated in Figure~\ref{fig:syn_multi_imbalance}(a)), the choice of target domain has a significant impact on the result. When we choose green as the target domain and map red and blue points to green points (Figure~\ref{fig:syn_multi_imbalance}(b)), 
although red and blue points are aligned with green points, they are still not overlapped as desired. This is because blue or red points tend to align along their boundaries due to the structure-preserving components. Although smaller $\alpha$ could solve the issue, the rule of thumb solution is choosing the domain with the most points as the target domain. For example, if we choose red points as the target domain and map green and blue points to the domain of the red point (Figure~\ref{fig:syn_multi_imbalance}(c)), the three-color datasets are well overlapped. 
The color feature are significantly removed with AUC from $0.77$ to $0.64$ (Table~\ref{table_binary_imbalance_multi}).

%\section{More Details on Real Data Experiments}
\section{More Experiments on Real Datasets}
We show more experiments for both multi-language embedding datasets and merchant embedding dataset. We conduct our experiments on a Red Hat Linux server with Intel Xeon E5-2650 v4 CPU and Nvidia Tesla P100 GPU.
\subsection{Multi-language Embedding Datasets}
\label{sec:multi-lang-more}
For multi-language embedding datasets, we demonstrate the results on more languages, including Greek (el), Vietnamese (vi), Arabic (ar), Czech (cs) and Dutch (nl).
This group of languages are less similar to English than those mentioned in the main paper. 
As the experiments in the main paper, we set the number of refinements as $0$ to compare the model only since refinement can be applied to all three models.
From Table \ref{table_nn_lang_more}, our model can outperform MUSE and UMWE on all the language pairs. 
For language pair el-en, en-vi, vi-en, ar-en, MUSE cannot find a valid mapping. Thus both NN and CSLS results are close to $0$. 
This is probably because el, vi and ar are from different families as en. 
UMWE can overcome this issue by mapping them at the same time, but both NN and CSLS are not as good as our model.
In conclusion, our model is very robust and can extend to any language families, while MUSE is limited to work on languages similar to English.

\subsection{Merchant Embedding Dataset}
\label{sec:mrch_freq}
In the main paper, we show that after mapping between different areas, the location feature can be removed and MCC feature is still retained in Table \ref{table_merchant}. In this section, we show that the frequency feature (F3) can be retained as well in Table \ref{table_merchant_frequency}. Both our algorithm and MUSE can significantly reduce the location feature while retaining the frequency feature; our algorithm significantly outperforms MUSE across all the location pairs. F3/F2 is increased from $10\%$ to $50\%$ under the MUSE algorithm, while our algorithm can increase from $43\%$ to $78\%$.

\begin{table*}[]
\caption{Results on multi-Language embedding for word translation. NN and CSLS are two evaluation approaches. We use precision as metric for $K=1,5,10$. G\_ is the proposed algorithm result, and M\_ is the MUSE baseline method and U\_ is the UMWE baseline method.}
\centering
\resizebox{0.85\textwidth}{!}{ % If your table exceeds the column or page width, use this command to reduce it slightly
\begin{tabular}{l||c|cc|cc|cc|cc|cc}
\hline
 &  & en-el & el-en & en-vi & vi-en & en-ar & ar-en & en-cs & cs-en & en-nl & nl-en\\ 
\hline
%\multirow{1}{*}{M\_NN\_R} & K@1 & 69.8 & 71.3 & 70.4 & 61.9 & 63.1 &59.6 & 29.1 & 41.5 & NA & NA \\
%\hline
\multirow{3}{*}{M\_NN} &K@1 & 13.87 & 0.00 & 0.00 & 0.07 & 12.47 & 0.00 & 24.73 & 41.67 & 49.07 & 45.53 \\
&K@5 & 31.13 & 0.00 & 0.13 & 0.07 & 26.33 & 0.07 & 42.00 & 58.33 & 67.80 & 61.87 \\
&K@10 & 38.33 & 0.00 & 0.33 & 0.07 & 32.27 & 0.07 & 49.67 & 64.40 & 73.33 & 67.00 \\
\hline
 \multirow{3}{*}{U\_NN} &K@1 & 18.73 & 26.27 & 3.27 & 1.87 & 14.60 & 22.49 & 26.87 & 31.13 & 43.07 & 33.67 \\
&K@5 & 36.47 & 44.80 & 8.40 & 5.60 & 32.00 & 38.35 & 46.53 & 48.00 & 60.20 & 48.93 \\
&K@10 & 43.27 & 50.53 & 10.73 & 8.53 & 38.87 & 44.51 & 53.20 & 53.07 & 66.07 & 54.13 \\
\hline
 \multirow{3}{*}{G\_NN} &K@1 & ${\bf 28.20 }$ & ${\bf 41.47 }$ & ${\bf 12.13 }$ & ${\bf 31.93 }$ & ${\bf 19.97 }$ & ${\bf 34.80 }$ & ${\bf 28.33 }$ & ${\bf 49.73 }$ & ${\bf 60.00 }$ & ${\bf 61.67}$ \\
&K@5 & ${\bf 46.60 }$ & ${\bf 59.93 }$ & ${\bf 23.27 }$ & ${\bf 45.33 }$ & ${\bf 41.45 }$ & ${\bf 51.74 }$ & ${\bf 50.27 }$ & ${\bf 67.73 }$ & ${\bf 76.40 }$ & ${\bf 75.60}$ \\
&K@10 & ${\bf 52.53 }$ & ${\bf 65.27 }$ & ${\bf 27.67 }$ & ${\bf 49.60 }$ & ${\bf 48.67 }$ & ${\bf 57.50 }$ & ${\bf 58.93 }$ & ${\bf 71.60 }$ & ${\bf 80.60 }$ & ${\bf 79.27}$ \\
\hline
\hline
%\multirow{1}{*}{M\_CSLS\_R} & K@1 & 75.7 & 79.7 & 77.8 & 71.2 & 70.1 &66.4 & 37.2 & 48.1 & 66.2 & 58.7 \\
%\hline
 \multirow{3}{*}{M\_CSLS} &K@1 & 22.67 & 0.00 & 0.00 & 0.00 & 15.00 & 0.00 & 31.07 & 47.53 & 59.67 & 55.33 \\
&K@5 & 42.93 & 0.00 & 0.07 & 0.07 & 32.60 & 0.07 & 52.80 & 65.53 & 77.27 & 70.93 \\
&K@10 & 50.80 & 0.00 & 0.07 & 0.07 & 39.00 & 0.07 & 60.07 & 70.67 & 82.73 & 75.00 \\
\hline
 \multirow{3}{*}{U\_CSLS} &K@1 & 25.20 & 34.47 & 6.27 & 4.20 & 18.47 & 28.45 & 32.93 & 38.53 & 50.67 & 43.67 \\
&K@5 & 44.00 & 54.33 & 13.07 & 10.93 & 37.20 & 46.92 & 53.67 & 55.67 & 67.60 & 57.93 \\
&K@10 & 50.33 & 59.07 & 16.27 & 14.93 & 44.07 & 52.95 & 61.07 & 60.20 & 72.67 & 63.33 \\
\hline
\multirow{3}{*}{G\_CSLS} &K@1 & ${\bf 32.40 }$ & ${\bf 45.80 }$ & ${\bf 21.80 }$ & ${\bf 38.33 }$ & ${\bf 23.93 }$ & ${\bf 36.81 }$ & ${\bf 34.13 }$ & ${\bf 53.60 }$ & ${\bf 67.47 }$ & ${\bf 68.67}$ \\
&K@5 & ${\bf 51.53 }$ & ${\bf 64.27 }$ & ${\bf 33.93 }$ & ${\bf 50.26 }$ & ${\bf 45.60 }$ & ${\bf 54.75 }$ & ${\bf 57.20 }$ & ${\bf 69.80 }$ & ${\bf 82.07 }$ & ${\bf 80.60}$ \\
&K@10 & ${\bf 57.87 }$ & ${\bf 69.47 }$ & ${\bf 38.33 }$ & ${\bf 54.86 }$ & ${\bf 52.28 }$ & ${\bf 59.71 }$ & ${\bf 64.27 }$ & ${\bf 74.47 }$ & ${\bf 85.53 }$ & ${\bf 83.20}$ \\
 \hline
\end{tabular}
}
\label{table_nn_lang_more}
\end{table*}

\begin{table*}[]
\caption{Results on Merchant Embedding Dataset. O\_ represents the original result, G\_ is the proposed algorithm result, and M\_ is the MUSE baseline. We report the AUC scores for frequency feature (F3) and location feature (F2).}
\centering
\resizebox{0.9\textwidth}{!}{ % If your table exceeds the column or page width, use this command to reduce it slightly
\begin{tabular}{l||ccc|ccc|ccc}
\hline
  & O\_F3  & O\_F2 &  O\_F3/O\_F2 & G\_F3 & G\_F2 & G\_F3/G\_F2 & M\_F3  & M\_F2 & M\_F3/M\_F2\\ 
\hline
LA$\to$SF    & 0.57 & 0.88 & 0.65 & 0.58 & 0.59 & ${\bf0.98}$ & 0.57 & 0.63 & 0.90 \\
SF$\to$LA    & 0.57 & 0.88 & 0.65 & 0.57 & 0.61 & ${\bf0.93}$ & 0.57 & 0.78 & 0.73 \\
LA$\to$CHI   & 0.59 & 0.95 & 0.62 & 0.59 & 0.57 & ${\bf1.04}$ & 0.59 & 0.71 & 0.83 \\
CHI$\to$LA   & 0.57 & 0.95 & 0.60 & 0.57 & 0.57 & ${\bf1.00}$ & 0.56 & 0.63 & 0.89 \\
SF$\to$CHI   & 0.57 & 0.93 & 0.61 & 0.57 & 0.59 & ${\bf0.97}$ & 0.57 & 0.79 & 0.72 \\
CHI$\to$SF   & 0.59 & 0.93 & 0.63 & 0.59 & 0.56 & ${\bf1.05}$ & 0.59 & 0.66 & 0.89 \\
MAN$\to$LA  & 0.57 & 0.9 & 0.63 & 0.56 & 0.54 & ${\bf1.04}$ & 0.57 & 0.82 & 0.70 \\
LA$\to$MAN  & 0.57 & 0.9 & 0.63 & 0.57 & 0.54 & ${\bf1.06}$ & 0.56 & 0.6 & 0.93 \\
MAN$\to$SF  & 0.58 & 0.88 & 0.66 & 0.59 & 0.53 & ${\bf1.11}$ & 0.58 & 0.62 & 0.94 \\
SF$\to$MAN  & 0.59 & 0.88 & 0.67 & 0.58 & 0.53 & ${\bf1.09}$ & 0.59 & 0.62 & 0.95 \\
MAN$\to$CHI  & 0.59 & 0.93 & 0.63 & 0.58 & 0.52 & ${\bf1.12}$ & 0.59 & 0.8 & 0.74 \\
CHI$\to$MAN  & 0.59 & 0.93 & 0.63 & 0.58 & 0.52 & ${\bf1.12}$ & 0.58 & 0.61 & 0.95 \\
\hline
\end{tabular}
}
\label{table_merchant_frequency}
\end{table*}

\section{Details on Real-world Applications}
%\subsection{Details for False Merchant Identity Detection}
\subsection{False Merchant Identity Detection}
\label{sec:mrch-emb}
In this section, we provide details about our model design for the system presented in the false merchant identity detection experiment section and additional experiment results showcasing the effectiveness of the proposed embedding alignment method for detecting merchants with false identities. 

\subsubsection{Model Design}
\label{sec:mcc-classifier}
The top part of Figure~\ref{fig:classifier} shows how the merchant category identification system interacts with various components within our payment ecosystem.
The system processes the incoming transactions in real-time and notifies the investigation team whenever a merchant is suspicious.
The internal merchant category identification system consists of two databases archiving various information and a core merchant classification model.
% Following~\cite{yeh2020merchant}, the core merchant classification model uses multi-modal design using both embedding information and time series information for better classification performance as shown in Figure~\ref{fig:classifier}.bottom.
The core merchant classification model uses a multi-modal design using both embedding information and time-series information for better classification performance as shown in the bottom part of  Figure~\ref{fig:classifier}.
The embedding information is processed with multilayer perceptron and the time-series information is processed with 1D convolutional net.

\begin{figure}
    \centering
  \includegraphics[width=0.8\linewidth]{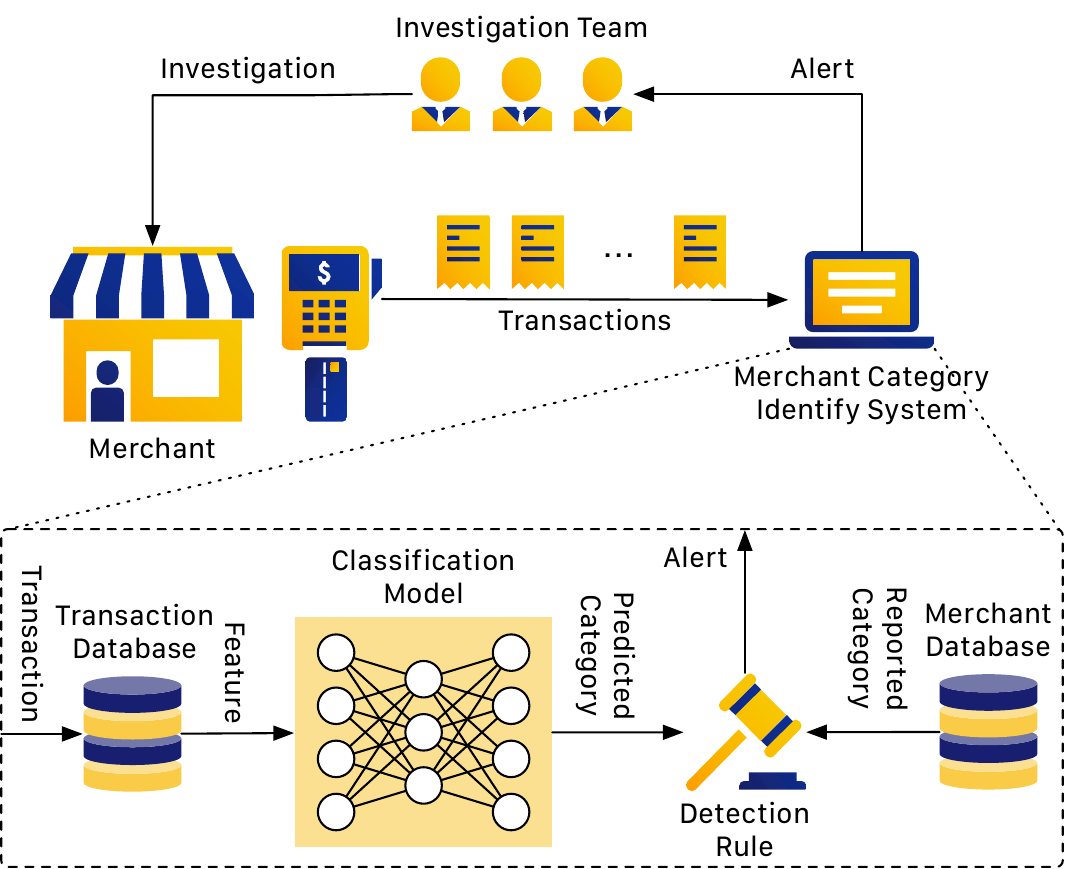}
  \includegraphics[width=0.8\linewidth]{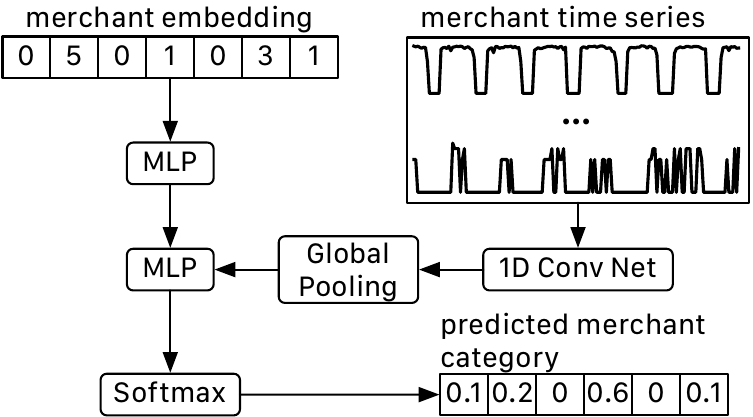}
  \caption{Overall system design and architecture design for our merchant category classifier.
  MLP stand for multilayer perceptron and the 1D convolutional net uses a design similar to the temporal convolutional network.}% proposed by~\protect\cite{bai2018empirical}.}
  \label{fig:classifier}
\end{figure}

\subsubsection{Additional Experiment Result}
\label{sec:mcc-result}
An accurate merchant false identity detection system is important for payment processing systems because a merchant could report a false merchant category to avoid scrutiny from banks and regulators.
For example, a high-risk merchant may pretend to be in a low-risk merchant category by reporting a fake merchant category to avoid higher processing fees associated with risky categories.
Specific business type (i.e., gambling) is only permitted in some regions and territories.

Because our goal is to detect merchants with false merchant category instead of classification, we further evaluate the accuracy of the complete detection system.
In our system, the particular detection rule we used is: if a merchant's self-reported merchant category is not within the top-$k$th most likely merchant category, the merchant will be reported as a suspicious merchant where $k$ is an adjustable threshold for our detection system.
To perform the evaluation, we randomly select $10\%$ of the test merchant and randomly change their self-reported merchant category to emulate the process of one merchant faking its merchant identity.
As we vary the detection threshold, we report the f1 score and the number of suspicious flagged merchants.
The experiment result is shown in Figure~\ref{fig:real_exp}.
Our attenuating method can generate better quality embeddings comparing to other methods.
The resulting merchant category identification system can capture suspicious merchants more accurately and also report less suspicious merchants to the investigation team than the system using raw or MUSE processed embeddings.

\begin{figure}
\centering
  \includegraphics[width=\linewidth]{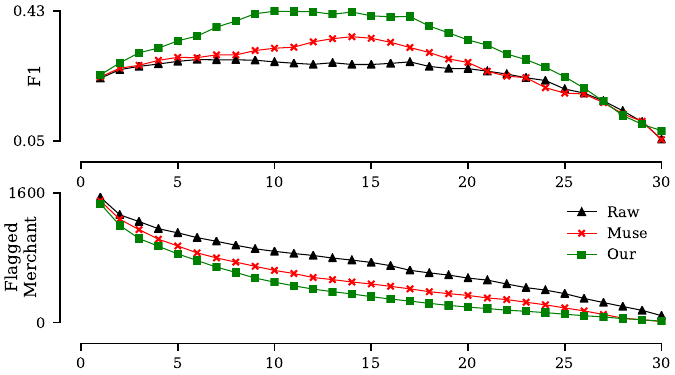}
  \caption{The performance of the merchant category identification system.}
  \label{fig:real_exp}
\end{figure}

\subsection{Cross-City Restaurant Recommendations}
\label{sec:rest-result}
To test the effectiveness of our algorithm under a large range of $\alpha$, we vary $\alpha$ from $0.5$ to $5$. All the alphas can work consistently well and $\alpha = 2$ gives the best results. Using $\alpha = 1$ as the rule of thumb can generally give good results.
\begin{table}[h]
\caption{Performance of the cross-city restaurant recommendations with different $\alpha$.}
\centering
%\resizebox{0.95\textwidth}{!}{ % If your table exceeds the column or page width, use this command to reduce it slightly
\begin{tabular}{l||c}
\hline
& Score \\ 
\hline
Raw data  &  60.36  \\
MUSE & 60.33 \\
$\alpha=5$  &  63.51 \\
$\alpha=2$  &  64.11 \\
$\alpha=1$&  63.60\\
$\alpha=0.5$&  63.51 \\
\hline
\end{tabular}
\label{table_cross_alpha}
\end{table}
